# Supplementary material for: Efficient Federated Low Rank Matrix Completion
Source: arXiv:2405.06569 source file (2024-09-30)
Supplement: Supplementary file 1 [file improved_lrmc_altgdmin_supplement.tex]

\section{Preliminaries}
\begin{enumerate}
\item \newtheorem*{theorem3.22}{Theorem 3.22 from \cite{Chen_2021}}
\begin{theorem3.22} For rank-$r$ $\mu$-incoherent $\X^* \in \mathbb{R}^{n_1 \times n_2}$, $n_2 \geq n_1$, $\X^* \svdeq \U^* \Sigma^* \V^{*\intercal}$. Suppose that $n_1p \geq C_1 \kappa^2 \mu r \log n_2$ for some sufficiently large Constant $C > 0$. Then, with probability exceeding $1 - O(n_2^{-10})$,
\begin{equation}
\max \{ \textrm{dist}(\U,\U^*), \textrm{dist} (\V,\V^*)\} \leq C \kappa \sqrt{\frac{\mu r \log n_2}{n_1p}}, \label{eq:initSmpl}
\end{equation}
where $\textrm{dist}(\U,\U^*) = \min_{\Q\Q^\intercal =  \Q^\intercal \Q = \I}\lV \U\Q -\U^*\rV_{op} =  \min_\Q\lV \U - \U^*\Q\rV_{op}$, and $\kappa$ is the condition number of $\X^*$.
\end{theorem3.22}
\item \newtheorem*{theorem4.1}{Theorem 4.1 from  \cite{lrpr_gdmin}}
\begin{theorem4.1}
[Wedin $\sin \Theta$ theorem for Frobenius norm subspace distance]
For two $n_1 \times n_2$ matrices $\A$, $\B$, let $\Ustar, \U$ denote the matrices containing their top $r$ singular vectors and let $\V^{*\intercal}, \V^\intercal$ be the matrices of their right singular vectors. Let $\sigma^*_r, \sigma^*_{r+1}$ denote the $r$-th and $(r+1)$-th singular values of $\A$.
If $\|\A - \B\| \le \sigma^*_r - \sigma^*_{r+1}$, then
\begin{equation}
\SE_F(\U, \Ustar)
\le \frac{\sqrt{2} \max(\|(\A - \B)^\top \Ustar\|_F, \|(\A - \B)^\top \V^{*\top}\|_F    )}{\sigma^*_r - \sigma^*_{r+1} - \lV \A - \B\rV_{op}}.
\label{eq:WdinSin}
\end{equation}
\label{Wedin_sintheta}
\end{theorem4.1}
%\item \newtheorem*{theorem3.22}{Theorem 3.22 from \cite{Chen_2021}}
\item \newtheorem*{Lemma}{Equations (9), (10) from  \cite{nashed1968decomposition}}
\begin{Lemma}
Let $\mathcal H$ be a real Hilbert space and let $\mathcal C$ be a closed convex set therein. Let $\Pi_\mathcal{C}$ denote the projection onto set $C$. That is, $\Pi_\mathcal{C}(\x)$ is the unique projection of $\x \in \mathcal H$  such that  $\lV \x  - \Pi_{\mathcal C}(\x) \rV \leq \lV \x -  \y \rV\, \forall \y \in \mathcal C$.
Then, for any $\x_1,\x_2 \in \mathcal H$,
\begin{equation}
\lV \Pi_{\mathcal C}(\x_1) - \Pi_{\mathcal C}(\x_2) \rV \leq \lV \x_1 - \x_2 \rV \label{eq:nonExp}
\end{equation}
%	For $\x_2 \in \mathcal C$ and $\x_1 \in \mathcal H$,
%	\begin{equation}
%		\lV \Pi_{\mathcal C}(\x_1) - \x_2 \rV \leq \lV \x_1 - \x_2 \rV. \label{eq:nonExpIdn}
%	\end{equation}
\end{Lemma}
\begin{proof}
%We first show that $\langle \y - \Pi_{\mathcal C} (\x),  \Pi_{\mathcal C}(\x) - \x \rangle \geq 0  \forall y \in \mathcal C$. %To see this, consider the line $y_t = ty + (1- t)\Pi_{\mathcal C}(\x) \forall 0 \leq t \leq 1$, and let $\y_t$ be a point on this line. By \eqref{eq:prj}, $ \lV \x - \Pi_{\mathcal C}(\x) \rV_2^2 \leq \lV  \y_t  - \Pi_{\mathcal C}(\x)  \rV_2^2$. Using $0 \leq \lV \x - \Pi_{\mathcal C}(\x) \rV_2^2$ and expanding $\lV  \y_t  - \Pi_{\mathcal C}(\x)  \rV_2^2 = \langle \y_t  - \Pi_{\mathcal C}(\x), \y_t  - \Pi_{\mathcal C}(\x) \rangle$,
%	\begin{equation}
%		 \langle \y_t  - \Pi_{\mathcal C}(\x), \y_t  - \Pi_{\mathcal C}(\x) \rangle \geq 0. \label{eq:prjThrmPrf}
%	\end{equation}
%	 Because $\y_t$ can be chosen to be any point in $\y \in \mathcal C$,
%	\begin{equation}
%		\langle \y  - \Pi_{\mathcal C}(\x), \y  - \Pi_{\mathcal C}(\x) \rangle \geq 0. \label{eq:prjThrmPrf}
%	\end{equation}

Let $\x^* = \Pi_{\mathcal C}(\x)$ denote the projection of $\x \in \mathcal H$ onto $\mathcal C$; such  $\x^*$  always exists, see section 3.12 of \cite{luenberger1997optimization}. We will first show  $\langle \x^* - \x, \y - \x^* \rangle \geq 0 \forall \y \in \mathcal C$.   Note that
\begin{equation}\x^*=\argmin_{\y \in \mathcal C} f(\y), f(\y) =  \frac{1}{2}\lV \x - \y   \rV_2^2.\end{equation}
By the first-order condition of optimality (eq (4.21) in \cite{boyd2004convex}),
\begin{equation} \x^* = \argmin_{\y \in \mathcal C} f(\y) \iff  \langle \nabla f(\x^*) , \y - \x^*\rangle \geq 0 \forall \y \in \mathcal C.\label{eq:optmlCndtn}\end{equation}
For $f(\y) = \frac{1}{2}\lV \y - \x \rV_2^2,  \nabla f_{\y} = \y - \x,$ and $\nabla f(\x^*)  = \x^* - \x$. Substituting in \eqref{eq:optmlCndtn},
\begin{equation}
\langle  \x^* - \x, \y - \x^*  \rangle \geq 0 \, \forall \y \in \mathcal C. \label{eq:varCnvx}
\end{equation}
To prove \eqref{eq:nonExp}, substitute $\x = \x_1$ and $\y = \x_2^*$ in \eqref{eq:varCnvx}
\begin{equation} \langle \x_1^* - \x_1, \x_2^* - \x_1^*\rangle \geq 0 \label{eq:stp1}, \end{equation}
where $\x_1^*(\x_2^*) \in \mathcal C$ denote the projection of $\x_1(\x_2) \in \mathcal H$.  Next, substitute $\x = \x_2$ and $\y = \x_1^*$ in \eqref{eq:varCnvx},
\begin{equation} \langle \x_2^* - \x_2, \x_1^* - \x_2^*\rangle \geq 0 \implies \langle \x_2 - \x_2^*, \x_2^* - \x_1^*\rangle \geq 0 \label{eq:stp2}. \end{equation}		
Adding \eqref{eq:stp1}, \eqref{eq:stp2},
\begin{align}	
& \langle \x_1^* - \x_2^* , \x_2^* - \x_1^* \rangle + \langle \x_2 - \x_1, \x_2^* - \x_1^* \rangle \geq 0\\
& \implies \langle \x_1^* - \x_2^*, \x_2^* - \x_1^* \rangle \geq - \langle \x_2 - \x_1, \x_2^* - \x_1^* \rangle\\
& \implies - \langle \x_1^* - \x_2^*, \x_2^* - \x_1^* \rangle \leq\langle \x_2 - \x_1, \x_2^* - \x_1^* \rangle\\
& \implies \langle \x_2^* - \x_1^*, \x_2^* - \x_1^* \rangle \leq\langle \x_2 - \x_1, \x_2^* - \x_1^* \rangle\\
& \implies \lV \x_2^* - \x_1^* \rV_2^2 \leq \lV \x_2 - \x_1 \rV \lV \x_2^* - \x_1^* \rV \label{eq:Cchy}\\
& \implies \lV \x_2^* - \x_1^* \rV_2 \leq \lV \x_2 - \x_1 \rV,
\end{align}
where \eqref{eq:Cchy} is by the Cauchy-Schwartz inequality. %\eqref{eq:nonExpIdn} follows by noting that for $\x_2 \in \C$, $\Pi_{\mathcal C}(\x_2) = \x_2$.		
For another proof of \eqref{eq:nonExp},  see equation (1.5) from \cite{zarantonello1971projections}.
\end{proof}
\item \newtheorem*{thrmMtrxBrnstn}{\textit{Matrix Ber}nstein, Theorem 5.4.1 from \cite{versh_book}}
\begin{thrmMtrxBrnstn} Let $\Z_1, \cdots, \Z_N$ be independent mean-zero $m \times n$ random matrices, such that $\lV \Z_i \rV \leq L \forall i$, almost surely. Then, for every $ t > 0$, we have
\begin{equation}
\Pr\big[\lV \sum_{i = 1}^{i = N } \Z_i \rV  \geq t \big] \leq  (m + n) \exp(-c \cdot \min(\frac{t^2}{\sigma^2},\frac{t}{L})), \label{eq:mtrxBrnstn}
\end{equation}
where $\sigma^2 = \max(\lV \E[\sum_{i=1}^{i=N} \Z_i\Z_i^\intercal] \rV, \lV \E[\sum_{i=1}^{i=N} \Z_i^\intercal \Z_i] \rV)$.
\end{thrmMtrxBrnstn}
\end{enumerate}

%\subsubsection{delete}
%Assuming the above bound on $\delta^{(t')}$ for all $t'=0,1,\dots, t$, we can use the above equation at each $t'$ to argue that
%\begin{align*}
%\|{\u}^{(t+1)}_j \|
%& \le (1 - \frac{0.15}{\kappa^2})^t \|{\u^j}^{(0)}\| + [1 + (1 - \frac{0.15}{\kappa^2}) + (1 - \frac{0.15}{\kappa^2})^2 + \dots + (1 - \frac{0.15}{\kappa^2})^t]  0.7 \|{\ustar{}^j}\| \\
%& \le (1 - \frac{0.15}{\kappa^2})^t \|{\u^j}^{(0)}\|+ \frac{0.7 \kappa^2}{0.15} \|{\ustar{}^j}\|
%\le  \|{\u^j}^{(0)}\| + 5 \kappa^2 \|{\ustar{}^j}\| \le C \kappa^2 \sqrt{r}  \mu \sqrt{r/n}
%\end{align*}
%where for the last bound we used $\|{\u^j}^{(0)}\| \le C \sqrt{r} \mu \sqrt{r/n}$ and Assumption \ref{incoh}

\subsection{OLD Proof of Lemma \ref{lemma:Ugrad}}
\label{subsec:gradUBnd}
The gradient with respect to $\U$ is
$\gradU = \sum_{jk}  \deltajk \e_j (\x_{jk} - \x^*_{jk})\b_k^\intercal.$
We will bound $\| \gradU \|$ by the Matrix-Bernstein inequality. Using $n \le q$ and \eqref{eq:elmntErrBnd},
\[
L = \max_\jk |\x_\jk - \xstar_\jk|  \max_k \|\b_k\| \le   2\mu_u (r/\sqrt{n})  \delta^{(t)} \sigmax \cdot \mu \sqrt{r/q} \sigmax \le  2\mu_u \mu (r^{3/2} / n) \delta^{(t)} \sigmaxTwo,
\]
where $\max_{jk} |\x_{jk} - \x^*_{jk}|$ is bounded below
\begin{align}\hspace{-1.5em}
|\e_j^\top(\X - \Xstar)\e_k| % = |\e_j^\top(\U (\B - \G) + (\U \U^\top \Xstar - \Xstar) )\e_k|
\le  \|\e_j^\top\U \| \|\B - \G\| + \|(\U \U^\top - \I)\Ustar\| \|\Bstar \e_k\|
\le \mu_u \sqrt{r/n} \sqrt{r} \delta^{(t)} \sigmax + \mu \sqrt{r/q} \delta^{(t)}  \sigmax
\le 2 \mu_u (r/\sqrt{n}) \delta^{(t)} \sigmax.
\label{eq:elmntErrBnd}
\end{align}

{\begin{align}\hspace{-1.5em}
|\e_j^\top(\X - \Xstar)\e_k| % = |\e_j^\top(\U (\B - \G) + (\U \U^\top \Xstar - \Xstar) )\e_k|
\le  \|\e_j^\top\U \| \|\B - \G\| + \|(\U \U^\top - \I)\Ustar\| \|\Bstar \e_k\|
\le \mu_u \sqrt{r/n}  \delta^{(t)} \sigmax + \mu \sqrt{r/q} \delta^{(t)}  \sigmax
\le 2 \mu_u (\sqrt{r/n}) \delta^{(t)} \sigmax.
\label{eq:elmntErrBnd}
\end{align}}
The variances are
\begin{align}
&\sigma_1^2
= p \sum_\jk (\x_\jk - \xstar_\jk)^2 \e_j \b_k^\top \b_k \e_j^\top %\le p \cdot q \cdot \tilde\mu^2 (r^2/n) \cdot \tilde\mu^2 (r/q) \delta^{(t)}{}^2 \sigmax^4 =  p \cdot \tilde\mu^4 (r^3/n) \delta^{(t)}{}^2 \sigmax^4
%\le p \|\b_k\|^2 \cdot \|\e_j\|^2 \sum_\jk (\x_\jk - \xstar_\jk)^2
\le  p \|\b_k\|^2 \|\X - \Xstar\|_F^2
\le p\mu^2(r/q) \sigmaxTwo \cdot  ( \delta^{(t)} \sqrt{r} \sigmax )^2
= p\mu^2(r^2/q) \delta^{(t)}{}^2 \sigma^{*4}_{\max}. \notag\\
&\sigma_2^2
= p \| \sum_\jk (\x_\jk - \xstar_\jk)^2 \e_j^\top \e_j \b_k\b_k^\top \|
%\le p \|\b_k\|^2 \| \sum_\jk (\x_\jk - \xstar_\jk)^2 \|
\le  p \|\b_k\|^2 \|\X - \Xstar\|_F^2  = \sigma_1^2. \notag
\end{align}
{
\begin{align}
&\sigma_1^2
= p \sum_\jk (\x_\jk - \xstar_\jk)^2 \e_j \b_k^\top \b_k \e_j^\top %\le p \cdot q \cdot \tilde\mu^2 (r^2/n) \cdot \tilde\mu^2 (r/q) \delta^{(t)}{}^2 \sigmax^4 =  p \cdot \tilde\mu^4 (r^3/n) \delta^{(t)}{}^2 \sigmax^4
%\le p \|\b_k\|^2 \cdot \|\e_j\|^2 \sum_\jk (\x_\jk - \xstar_\jk)^2
\le  p \|\b_k\|^2 \|\X - \Xstar\|_F^2
\le p\mu^2(r/q) \sigmaxTwo \cdot  ( \delta^{(t)} \sigmax )^2
= p\mu^2(r/q) \delta^{(t)}{}^2 \sigma^{*4}_{\max}. \notag\\
&\sigma_2^2
= p \| \sum_\jk (\x_\jk - \xstar_\jk)^2 \e_j^\top \e_j \b_k\b_k^\top \|
%\le p \|\b_k\|^2 \| \sum_\jk (\x_\jk - \xstar_\jk)^2 \|
\le  p \|\b_k\|^2 \|\X - \Xstar\|_F^2  = \sigma_1^2. \notag
\end{align}}
Setting $t = \eps p \sqrt{r}  \delta^{(t)} \sigmaxTwo $, we have
\[
\frac{t^2}{\sigma^2} = \frac{\eps^2 p^2 r \delta^{(t)}{}^2 \sigmaxFour}{p \mu^2(r^2/q) \delta^{(t)}{}^2 \sigmaxFour}  = \frac{\eps^2 p q}{\mu^2 r} \leq \frac{\eps^2 p q}{\mu_u\mu r},
\ \
\frac{t}{L} = \frac{ \eps p \sqrt{r}  \delta^{(t)} \sigmaxTwo}{\mu_u\mu (r^{3/2} / n) \delta^{(t)} \sigmaxTwo} =  \frac{ \eps p n }{\mu_u\mu r}.
\]
By matrix Bernstein, for $\eps \leq 1$, w.p. at least $1 - \exp(\log q - \eps^2 p n  /\mu_u \mu r) $,
\[
\|\gradU - \E[\gradU] \| \le \eps p \sqrt{r}  \delta^{(t)} \sigmaxTwo.
\]
If $p > \mu_u \mu r \max(\log q, \log n )  / n \eps^2$, then the above bound holds w.p. at least $1 - 1/n^3$. Also,
\[
\E[\gradU] = p (\X- \Xstar) \B^\top,  %\ \ \|\E[\gradU] \| \le p \sqrt{r} \delta^{(t)} \sigmax^2.
\]

{Setting $t = \eps p   \delta^{(t)} \sigmaxTwo $, we have
\[
\frac{t^2}{\sigma^2} = \frac{\eps^2 p^2  \delta^{(t)}{}^2 \sigmaxFour}{p \mu^2(r/q) \delta^{(t)}{}^2 \sigmaxFour}  = \frac{\eps^2 p q}{\mu^2 r} \leq \frac{\eps^2 p q}{\mu_u\mu r},
\ \
\frac{t}{L} = \frac{ \eps p   \delta^{(t)} \sigmaxTwo}{\mu_u\mu (r / n) \delta^{(t)} \sigmaxTwo} =  \frac{ \eps p n }{\mu_u\mu r}.
\]
By matrix Bernstein, for $\eps \leq 1$, w.p. at least $1 - \exp(\log q - \eps^2 p n  /\mu_u \mu r) $,
\[
\|\gradU - \E[\gradU] \| \le \eps p   \delta^{(t)} \sigmaxTwo.
\]
If $p > \mu_u \mu r \max(\log q, \log n )  / n \eps^2$, then the above bound holds w.p. at least $1 - 1/n^3$. Also,
\[
\E[\gradU] = p (\X- \Xstar) \B^\top,  \ \ \|\E[\gradU] \| \leq p \lV \X - \X^* \rV \lV \B \rV  \leq C p \delta^{(t)} \sigmaxTwo,
\]
where we have used Lemma \ref{Berr_implic} above to bound $\lV \X - \X^* \rV_F \leq C \delta$.
}
 
\subsection{OLD Proof of Lemma \ref{lem:rowIncoh}}
\label{subsec:rowIncohProof}
Let $\gradUj \in \mathbb{R}^{1 \times r}$ denote the gradient of $\U \in \mathbb{R}^{n \times r}$ with respect to row $j$. We note the following
\begin{align}
& \gradUj = \sum_k \delta_k (\x_\jk - \xstar_\jk) \b_k^\top,
%\E[\gradU_j] = p \e_j^\top(\U \B \B^\top - \Ustar \Bstar \B^\top) ,
\ \|\E[\gradU_j] \| \lesssim 2 p \|\u_j\|  \sigmax^2.\notag\\
& L =  \max_k |\x_\jk - \xstar_\jk|  \max_k \|\b_k\| \le  \max( \max_k |\x_\jk| , \max_k |\xstar_\jk|)  \max_k \|\b_k\| \le \|\u_j\|||\b_k||^2  \le \|\u_j\|  \mu^{*2} (r/q) \sigmaxTwo. \notag\\
&\sigma_1^2
= \lV \sum_k p (\x_\jk - \xstar_\jk)^2 \b_k^\top \b_k \rV
\le  2p \lV \sum_k \u_j^\top \b_k \b_k^\top \u_j  \b_k^\top \b_k \rV \le 2p \max_k ||\b_k||^2  \u_j^\top (\sum_k \b_k \b_k^\top ) \u_j
\le 2p  ||\u_j||^2 \mu^{*2} (r/q) \sigmaxFour. \notag \\
&\sigma_2^2
= \lV \sum_k p (\x_\jk - \xstar_\jk)^2 \b_k\b_k^\top \rV
\le  2p \lV  \sum_k \u_j^\top \b_k \b_k^\top \u_j  \b_k\b_k^\top \rV  \le   2p\max_k || \b_k||^2  \lV \u_j^\top (\sum_k \b_k \b_k^\top ) \u_j \rV \notag \le 2p  ||\u_j||^2 \mu^{*2} (r/q) \sigmaxFour. \notag
\end{align}
Here, $\sigma_1^2 \equiv \E[\sum_k \delta_k (\x_{jk} - \x^*_{jk})^2\b_k^\intercal\b_k]$
and $\sigma_2^2 \equiv \E[\sum_k \delta_k (\x_{jk} - \x^*_{jk})^2\b_k\b_k^\intercal]$. By the matrix Bernstein inequality with $t = \eps p  \|\u_j\|  \sigmin^2$, we have
w.p. at least  $1 - \exp(\log q - \eps^2 p n /\mu^{*2} \kappa^4 r )$,
\begin{equation}
\|\E[\gradU_j] - \gradU_j \| \le \eps p  \|\u_j\|  \sigmin^2. \label{eq:gradUjBnd}
\end{equation}
This completes the proof for the first part of the lemma.  By line 5 of Algorithm 1, for $t = 0$, we have
\[
\tilde{\u}^{(1)^\top}_j  =
%\R^{-1}
\u_j^{(0)\top}  ( \I - \eta p \B \B^\top) + \eta p \ustar_j{}^\top  \Bstar \B^\top + \eta (\E[\gradU_j] - \gradU_j),
\]
where we have also added and subtracted the term $\eta \E[\gradU_j]$. Setting  $\eta < 0.5 / p \sigmax^2$  and assuming  $\delta^{(t)} \leq c/\kappa$ in Lemma \ref{:impli} gives $\sigma_{\min}^2(\B) \geq c' \sigmin^2$, ensuring that $\I - \eta p \B \B^\top$ is p.s.d. Therefore,  $\|\I - \eta p \B \B^\top\|  = 1 - \eta p \sigma_{\min}^2(\B) \leq  1 - c \eta p \sigmin^2$. Next,  bounding $\eta (\E[\gradU_j] - \gradU_j) \leq  \epsilon \eta p \lV \u_j \rV_2^2 \sigmin^2$ by \eqref{eq:gradUjBnd},
\begin{equation}
\|\tilde{\u}^{(1)}_j \|
\le \|\u_j^{(0)}\| (1 - \eta p \sigmin^2) + \eps \eta p \sigmin^2 \|\u_j^{(0)}\|   + \eta p \|\ustar_j\| \sigmax^2
\le \|\u_j^{(0)}\| (1 - \eta p \sigmin^2 (1-\eps))    + \eta p \sigmax^2 \|\ustar_j\|.
\label{eq:uTildeBnd}
\end{equation}
We bound $ \|\u^{(1)}_j\| \le \| (\R^{(1)})^{-1} \|  \| \tilde{\u}^{(1)}_j \| \rV$,  where $\tilde \U^{(t+1)} \overset{\text{QR}}{=} \U^{(1)} \R^{(1)}$,
\begin{equation}
\lV (\R^{(1)})^{-1} \rV = 1/\sigma_{\min}(\U - \eta  \lV f(\U,\B) \rV )
\leq  1/(1 - \eta p (1 + \epsilon) \sqrt{r} \delta^{(0)} \sigma_{\max}^{*2})
\leq 1/(1 - 0.25\eta p  \sigmin^2)
\leq 1 + \frac{1}{2} \eta p  \sigmin^2,  \label{eq:RinvBnd}
\end{equation}
%\begin{align}
%\lV (\R^{(1)})^{-1} \rV_{op} &= \frac{1}{\sigma_{\min}(\U - \eta  \lV f(\U,\B) \rV )}\notag\\
%&\leq \frac{1}{1 - \eta  \lV f(\U,\B)\rV_{op}} \notag \\
%&\leq  \frac{1}{1 - \eta p (1 + \epsilon) \sqrt{r} \delta_t \sigma_{\max}^{*2}}, \notag\\
%&\leq \frac{1}{1 - \eta p(1 + \eps)c_0 \sigmin^2 } && \because \delta_t \le  c_0/ (\sqrt{r} \kappa^2)\\
%&\leq \frac{1}{1 - 0.25\eta p  \sigmin^2} && (\text{Substituting }\delta_t \leq \frac{1}{4(1+ \eps)\sqrt r \kappa^2})\notag\\
%&\leq 1 + \frac{1}{2} \eta p  \sigmin^2, && (\text{For }\eta \leq \frac{1}{2 p\sigmin^{2}} ) \label{eq:RinvBnd}
%\end{align}
where we have substituted the upper bound on $\lV f(\U,\B) \rV$ from Lemma \ref{lemma:Ugrad}, assuming  $\delta^{(0)} \leq 1/{4(1+ \eps)\sqrt r \kappa^2}$ and used $1/(1-x) \leq 1 + 2x \, \forall x \leq 1/2$. Substituting \eqref{eq:uTildeBnd} and \eqref{eq:RinvBnd} in $\|\u^{(1)}_j\| \le \| (\R^{(1)})^{-1} \|  \| \tilde{\u}^{(1)}_j \|$,
\begin{equation}
\|\u^{(1)}_j\|
\le  (1 - \frac{1}{2} \eta p \sigmin^2) \|\u_j^{(0)}\|  \ + \  (1 + \frac{1}{2}\eta p \sigmin^2  ) \eta p \sigmax^2 \|\ustar_j\|,
\label{eq:uPosBnd}
\end{equation}
where we have  bounded $(1 + \frac{1}{2}\eta p \sigmin^2) (1 - \eta p \sigmin^2(1 - \epsilon) ) \leq  1 -\frac{1}{2}\eta p \sigmin^2$.  Setting $\eta = 0.5 / p \sigmax^2$,
\begin{equation}
\|\u^{(1)}_j\|
\le  (1 - c_1/\kappa^2)   \|\u_j^{(0)}\| +  0.7 \|\ustar_j\|.
\label{eq:rowIncoh_t}
\end{equation}
Assuming $\delta^{(t)} \leq c/(\sqrt{r}\kappa^2), \lV \v_k^{(t)} \rV \leq \tilde \mu \sqrt{r/q}$, we also have
\begin{equation}
\|\u^{(t+1)}_j\|
\le  (1 - c_1/\kappa^2)   \|\u_j^{(t)}\| +  0.7 \|\ustar_j\|,
\end{equation}
from which the following bound for any $t \geq 0$ follows
\begin{align}
\|\u^{(t)}_j\|
= (1 - c_1/\kappa^2)^{t}   \|\u_j^{(0)}\| + \frac{7}{10}\sum_{l=0}^{l = t - 1} (1- c_1/\kappa^2)^{l}\lV \u_j^* \rV_2 \leq \lV \u_j^{(0)} \rV_2 + \frac{1}{c_1} \kappa^2 \lV \u_j^* \rV_2,
\label{eq:rowIncoh_Time}
\end{align}
where recall from \eqref{eq:rowIncoh_t} that $c_1 = 0.25$.

\subsection{OLD Proof of Lemma \ref{lem:BIncohLmma}}
\label{subsec:bkIncoh}
We have
\begin{equation}
\b_k = \underbrace{(\U_k^\intercal\U_k)^{-1}}_{T_1} \underbrace{\U_k^\intercal \Ustar_k}_{T_2} \bstar_k.
\label{eq:bk}
\end{equation}
The following has been proved in Lemma C.6 of  \cite{lowrank_altmin}.
If $p \geq C\frac{\mu_u^2 r}{n \epsilon^2 }(\log n  + \log r)$, then  with probability greater than $1 - \frac{1}{n^3}$,
\begin{equation}
\| (\U_k^\intercal \U_k)^{-1} \| \leq  \frac{1}{(1 - \epsilon)p}. \label{eq:opBndTrm1Fnl}
\end{equation}
Consider the second term, $T_2$.  The term $\| T_2 - \E[T_2] \|$ can be bounded by the Matrix-Bernstein inequality \eqref{eq:mtrxBrnstn}. sWe have $\E[T_2] = p \U^\intercal \U^* \neq p \I$. By the reverse triangle inequality,
\begin{align}
\| \U_k^\intercal \Ustar_k - p \U^\intercal \U^* \|	 \geq \| \U_k^\intercal \Ustar_k \| - p,
\end{align}
where we have used $\| \U^\intercal \U^* \| \leq \| \U \| \| \U^* \| \leq 1$. Therefore,
\begin{equation}
\| \U_k^\intercal \Ustar_k \| \leq \| \U_k^\intercal \Ustar_k - p \U^\intercal \U^* \|_{op } + p.
\label{eq:rvsTrngleIcoh}
\end{equation}
Also, $T_2 - \E[T_2]$ is not symmetric. The variance $\sigma^2$ is now
$$\sigma^2 = \max(\| \sum_j \E [\Z_j \Z_j^\intercal] \|, \| \sum_j \E[\Z_j^\intercal \Z_j]\| ),$$
where $\Z_j = (\deltajk - p){\u^j} {\u^j}^{*\intercal}$, and
\begin{align}
&\E[\Z_j] = 0 \notag,\\
&\|  \Z_j \| = \max(1-p,p) \| {\u^j} \| \| {\u^j}^* \| \leq \mu_u\mu \frac{r}{n}, \notag\\
& \Z_j\Z_j^\intercal \sim
\begin{cases}
(1-p)^2 \| {\u^j}^* \|^2 {\u^j} {\u^j}^\intercal  & \text{w.p. } p\\
p^2 \| {\u^j}^* \|^2 {\u^j} {\u^j}^\intercal & \text{w.p. } 1-p,
\end{cases} \notag\\
& \Z_j^\intercal \Z_j \sim
\begin{cases}
(1-p)^2 \| {\u^j} \|^2 {\u^j}^* {\u^j}^{*\intercal}  & \text{w.p. } p\\
p^2 \| {\u^j} \|^2 {\u^j}^{*} {\u^j}^{*\intercal} & \text{w.p. } 1-p,
\end{cases} \notag
\end{align}
%The bound on the variance $\sigma^2$ in \eqref{eq:varBndT2} follows from
Both variances $\sigma^2(\Z_j \Z_j^\intercal)$ and $\sigma^2(\Z_j^\intercal \Z_j)$ can be bounded by the same upper bound. Note that \begin{align}
\E[\Z_j\Z_j^\intercal] &= p(1-p)^2 \| {\ustar{}^j} \|^2 {\u^j}{\u^j}^\intercal + p^2(1-p)\| {\ustar{}^j} \|^2 {\u^j} {\u^j}^\intercal \notag \\ &\triangleq p' \| {\u^j}^* \|^2 {\u^j} {\u^j}^\intercal,  \enskip \text{ where }  p' = p(1-p)^2 + p^2(1-p) \leq 2p.  \end{align}
The variance $\sigma^2(\Z_j \Z_j^\intercal) = \| \sum_{j=1}^{j=n} \E[\Z_j\Z_j^\intercal] \| =  p' \|   \sum_{j=1}^{j=n} \| {\u^j}^* \|^2   ({\u^j} {\u^j}^\intercal) \|  = p' \max_{\| \w \| = 1}  \sum_{j=1}^{j=n} \w^\intercal (\| {\u^j}^* \|^2 {\u^j} {\u^j}^\intercal)$ is
\begin{align}
	&\sigma^2(\Z_j \Z_j^\intercal) =     p' \max_{\lV \w \rV = 1}  \sum_{j=1}^{j=n} \w^\intercal (\| {\u^j}^* \|^2 {\u^j} {\u^j}^\intercal)\w  \leq  p' \mu^2 \frac{r}{n} \max_{\lV \w \rV = 1} \w^\intercal  \sum_{j=1}^{j=n}   {\u^j} {\u^j}^\intercal\w \notag\\
	 & = p' \mu^2 \frac{r}{n} \max_{\lV \w \rV = 1 } \w^\intercal  \U^\intercal\U \w = p' \mu^2\frac{r}{n} \max_{\w} \w^\intercal \w = p' \mu^2 \frac{r}{n} \leq 2p \mu^2 \frac{r}{n}.
\end{align}
\begin{comment}
\begin{align}
\sigma^2(\Z_j \Z_j^\intercal)	& =  \| \sum_{j=1}^{j=n} \E[\Z_j\Z_j^\intercal] \| =  p' \|   \sum_{j=1}^{j=n} \| {\u^j}^* \|^2   ({\u^j} {\u^j}^\intercal) \| \notag \\
&= p' \max_{\w \colon \| \w \| = 1}  \sum_{j=1}^{j=n} \w^\intercal (\| {\u^j}^* \|^2 {\u^j} {\u^j}^\intercal) \w \notag \\
&\leq p' \mu^2 \frac{r}{n} \max_{\w \colon \| \w \| = 1} \w^\intercal  \sum_{j=1}^{j=n}   {\u^j} {\u^j}^\intercal \w \notag \\
&\leq p' \mu^2 \frac{r}{n} \max_{\w \colon \| \w \| = 1} \w^\intercal  \U^\intercal\U \w \notag\\
& = p' \mu^2\frac{r}{n} \max_{\w} \w^\intercal \w \notag \\
&= p' \mu^2 \frac{r}{n} \leq 2p \mu^2 \frac{r}{n} \notag.
\end{align}
\end{comment}
$\sigma^2(\Z_j^\intercal \Z_j)$ can be similarly bounded as $\sigma^2(\Z_j^\intercal \Z_j) \leq 2p \mu_u^{2}\frac{r}{n}$. Because $\mu_u \geq \mu$, we have $\sigma^2(\Z_j \Z_j^\intercal) \geq \sigma^2(\Z_j^\intercal \Z_j)$. %Analogous to \eqref{eq:T1EpsBnd},
By the Matrix-Bernstein inequality \eqref{eq:mtrxBrnstn}, for $\epsilon \leq 2$ and w.p. greater than $1 - \exp(\log 2 r - c \frac{n \epsilon^2 p}{\mu_u^2 r})$
\begin{equation}
\| \U_k^\intercal \Ustar_k - p \U^\intercal \U^* \| \leq \epsilon p.
\label{eq:mtrxBrnstnIncoh}
\end{equation}
From \eqref{eq:rvsTrngleIcoh} and \eqref{eq:mtrxBrnstnIncoh},  w.h.p,
\begin{equation}
\| \U_k^\intercal \U^*_k \| \leq (1 + \epsilon)p. \label{eq:T2_incoh_bnd}
\end{equation}
Substituting \eqref{eq:opBndTrm1Fnl},  \eqref{eq:T2_incoh_bnd} in \eqref{eq:bk}, and setting $\epsilon =1/10$, we have
\begin{equation}
\| \b_k \| \leq \frac{3}{2} \| \bstar_k \| \leq \frac{3}{2}\sigmax \mu \sqrt{r/q}.
\end{equation}
