# Supplementary material for: Efficient Federated Low Rank Matrix Completion
Source: arXiv:2405.06569 source file (2024-09-30)
Supplement: Supplementary file 2 [file supplement_SPL_lrmc_altgdmin.pdf]

# APPENDIX A
# MAIN LEMMAS AND PROOF OF THEOREM 4.1

## A. Definitions

Recall that $\delta^{(t)} = \mathrm{SD}_2(\boldsymbol{U}^{(t)}, \boldsymbol{U}^*)$. Let $\boldsymbol{G} \equiv \boldsymbol{G}^{(t)} = (\boldsymbol{U}^{(t)})^\intercal \boldsymbol{X}^\star$, $\boldsymbol{U} \equiv \boldsymbol{U}^{(t)}$, $\boldsymbol{B} \equiv \boldsymbol{B}^{(t+1)}$, and $\boldsymbol{X} \equiv \boldsymbol{X}^{(t)} = \boldsymbol{U}^{(t)}\boldsymbol{B}^{(t+1)}$. Also let $\boldsymbol{U}^+ \equiv \boldsymbol{U}^{(t+1)}$. Let $\xi_{jk} \overset{\text{iid}}{\sim} Bernoulli(p)$ for all $j \in [n], k \in [q]$. Thus $\Omega_k = \{j : \xi_{jk} = 1\}$ is the set of indices of the observed entries in column $k$. Recall that $\boldsymbol{S}_k = \boldsymbol{I}_{\Omega_k}{}^\intercal$ and $\boldsymbol{U}_k := \boldsymbol{S}_k \boldsymbol{U}$. Let $\mu_u := C\mu\sqrt{r}$.

## B. Lemmas

All lemmas below assume Assumption 1.1 (singular vectors' incoherence) holds.

**Lemma A.1.** *(Initialization [2, Lemma C.1 and C.2]) Assume $p \geq C\kappa^6(\mu)^4 r^6/n$. Then, w.p. at least $1 - 1/n^3$, we have*

1) $\mathrm{SD}_2(\boldsymbol{U}^{(0)}, \boldsymbol{U}^*) \leq c/(\sqrt{r}\kappa^2)$.
2) $\boldsymbol{U}^{(0)}$ *is incoherent with parameter $\mu_u := C\mu\sqrt{r}$, that is, $\|\boldsymbol{u}^{j\,(0)}\| \leq \mu_u\sqrt{\frac{r}{n}}$ for all $j \in [n]$.*

**Lemma A.2.** *[2, Lemma C.8] Assume $\|\boldsymbol{u}^j\| \leq \mu_u\sqrt{\frac{r}{n}}$ and $p \geq C\mu^2\mu_u^2 r^2\kappa^4/n$, $\delta^{(t)} < c/\sqrt{r}\kappa^2$. Then, w.p. greater than $1 - 1/n^3$, $\|\boldsymbol{B} - \boldsymbol{G}\|_F \leq \delta^{(t)}\sqrt{r}\sigma^*_{\max}$.*

**Lemma A.3.** *Assume $\|\boldsymbol{B} - \boldsymbol{G}\|_F \leq \delta^{(t)}\sqrt{r}\sigma^*_{\max}$. Then,*

1) $\|\boldsymbol{X} - \boldsymbol{X}^\star\|_F \leq 2\delta^{(t)}\sqrt{r}\sigma^*_{\max}$.
2) $\|\boldsymbol{B}\| \leq (1 + \delta^{(t)}\sqrt{r})\sigma^*_{\max}$.
3) $\sigma_{\min}(\boldsymbol{B}) \geq \sqrt{1 - \delta^{(t)2}}\sigma^*_{\min} - \delta^{(t)}\sigma^*_{\max}$.

**Lemma A.4.** *Assume $\|\boldsymbol{u}^j\| \leq \mu_u\sqrt{r/n}$ and $p \geq C\frac{\mu_u^2 r}{n\epsilon^2}(\log n + \log r)$. Then, w.p. greater than $1 - 1/n^3$, $\|\boldsymbol{b}_k\| \leq 2\sigma^*_{\max}\mu\sqrt{\frac{r}{q}}$.*

**Lemma A.5.** *Assume $\delta^{(t)} < c/\sqrt{r}\kappa^2$, $\|\boldsymbol{B} - \boldsymbol{G}\|_F \leq \delta^{(t)}\sqrt{r}\sigma^*_{\max}$, $\|\boldsymbol{u}^j\| \leq \mu_u\sqrt{r/n}$, $\|\boldsymbol{b}_k\| \leq \sigma^*_{\max}\mu\sqrt{r/q}$, and $p \geq C\frac{\mu_u\mu}{n\epsilon^2}r(\log n + \log q)$. Then,*

1) $\|\mathrm{GradU} - \mathbb{E}[\mathrm{GradU}]\| \leq \epsilon p\sqrt{r}\delta^{(t)}\sigma^{*2}_{\min}$ *w.p. greater than $1 - 1/n^3$,*
2) $\mathbb{E}[\mathrm{GradU}] = p(\boldsymbol{X} - \boldsymbol{X}^\star)\boldsymbol{B}^\intercal$ *and so* $\|\mathbb{E}[\mathrm{GradU}]\| \leq p\sqrt{r}\delta^{(t)}\sigma^{*2}_{\max}$.

**Lemma A.6.** *Assume $\delta^{(t)} < c/\sqrt{r}\kappa^2$, $\|\boldsymbol{B} - \boldsymbol{G}\|_F \leq \delta^{(t)}\sqrt{r}\sigma^*_{\max}$, $\|\boldsymbol{b}_k\| \leq \sigma^*_{\max}\mu\sqrt{r/q}$, and $p \geq C\mu^2 r\max(\log q, \log n)/n$. Then, w.p. greater $1 - 1/n^3$,*

1) $\|\mathrm{Grad}\boldsymbol{u}^j - \mathbb{E}[\mathrm{Grad}\boldsymbol{u}^j]\| \leq 0.1p\|\boldsymbol{u}^j\|\sigma^{*2}_{\max}$ *and*
2) $\|\boldsymbol{u}^{j\,(t)}\| \leq (1 - 0.15/\kappa^2)\|(\boldsymbol{u}^{j\,(t-1)})\| + 0.7\|\boldsymbol{u}^{*j}\|$.

*Proof.* The first two lemmas are taken from [2]. The last four are proved using matrix Bernstein [24, Theorem 5.4.1] and some linear algebra tricks borrowed from [21]. The proofs are given in Appendix B in longer version of this work [23]. □

## C. Proof of Theorem 4.1

We prove the following claim by induction. For all times $\tau \geq 0$, (i) $\delta^{(\tau)} \leq c/\sqrt{r}\kappa^2$ and $\delta^{(\tau)} \leq (1 - c/\kappa^2)\delta^{(\tau-1)}$; (ii) $\|\boldsymbol{u}^{j\,(\tau)}\| \leq \mu_u\sqrt{r/n}$; (iii) $\|\boldsymbol{B}^{(\tau+1)} - \boldsymbol{G}^{(\tau+1)}\|_F \leq \delta^{(\tau)}\sqrt{r}{\sigma^*_{\max}}^2$; and (iv) $\|\boldsymbol{b}_k^{(\tau+1)}\| \leq 1.1\mu\sqrt{r/q}\sigma^*_{\max}$. Theorem 4.1 is the first claim of this result.

*Base case:* let $\delta^{(-1)} = 1$. Lemma A.1 shows that $\delta^{(0)} \leq c/\sqrt{r}\kappa^2$ and $\|\boldsymbol{u}^{j\,(0)}\| \leq C\sqrt{r}\mu\sqrt{r/n} = \mu_u\sqrt{r/n}$. Since $c/\sqrt{r}\kappa^2 < 1/2$, this implies that $\delta^{(0)} \leq (1 - c/\kappa^2)\delta^{(-1)}$. This proves (i) and (ii) for $\tau = 0$. Lemmas A.2 and A.4 then prove (iii) and (iv) for $\tau = 0$.

*Induction assumption:* Assume the claim for $\tau = 1, 2, \ldots, t$.

*Induction step:* We use the last five lemmas and the induction assumption to prove the claim for $\tau = t + 1$. The induction assumption implies that Lemma A.6 applies for all $\tau = 1, 2, \ldots, t$. Using it and the base case, $\|\boldsymbol{u}^{j\,(0)}\| \leq \mu_u\sqrt{r/n}$ and for all $\tau = 1, 2, \ldots, t$,

$$\|\boldsymbol{u}^{j\,(\tau)}\| \leq (1 - 0.15/\kappa^2)\|\boldsymbol{u}^{j\,(\tau-1)}\| + 0.7\|\boldsymbol{u}^{*j}\|$$

Applying this for each $\tau = 0, 1, \ldots, t$, $\|\boldsymbol{u}^{j\,(t)}\| \leq (1 - \frac{0.15}{\kappa^2})^t\|\boldsymbol{u}^{j\,(0)}\| + [1 + (1 - \frac{0.15}{\kappa^2}) + \cdots + (1 - \frac{0.15}{\kappa^2})^{t-1}]0.7\|\boldsymbol{u}^{*j}\| \leq (1 - \frac{0.15}{\kappa^2})^t\|\boldsymbol{u}^{j\,(0)}\| + \frac{0.7\kappa^2}{0.15}\|\boldsymbol{u}^{*j}\| \leq \|\boldsymbol{u}^{j\,(0)}\| + 5\kappa^2\|\boldsymbol{u}^{*j}\| \leq C\kappa^2\sqrt{r}\mu\sqrt{r/n} := \mu_u\sqrt{r/n}$. Thus, $\|\boldsymbol{u}^{j\,(t)}\| \leq \mu_u\sqrt{r/n}$, i.e. (ii) holds for $\tau = t$.

Using this and the induction assumption bound on $\|\boldsymbol{B} - \boldsymbol{G}\|_F$ and $\|\boldsymbol{b}_k\|$ for $\tau = t$, Lemma A.5 applies. Using it, $\mathbb{E}[\mathrm{GradU}] = p(\boldsymbol{U}\boldsymbol{B} - \boldsymbol{X}^\star)\boldsymbol{B}^\intercal$, $\|\mathbb{E}[\mathrm{GradU}]\| \leq p\sqrt{r}\delta^{(t)}{\sigma^*_{\max}}^2$, and, if $p \geq C\frac{\mu_u\mu r}{n\epsilon^2}(\log n + \log q)$, then $\|\mathrm{GradU} - \mathbb{E}\mathrm{GradU}\| \leq \epsilon p\sqrt{r}\delta^{(t)}\sigma^{*2}_{\max}$. Set $\epsilon = 0.1/\sqrt{r}\kappa^2$. Then, $\|\mathrm{GradU} - \mathbb{E}\mathrm{GradU}\| \leq 0.1p\delta^{(t)}\sigma^{*2}_{\min}$ if $p \geq C\frac{\kappa^4\mu_u\mu r^2}{n}(\log n + \log q)$, We use this

to bound $\delta^{(t+1)} := \text{SD}_2(\boldsymbol{U}^+, \boldsymbol{U}^*)$ is bounded as follows. Let $\boldsymbol{P} := \boldsymbol{I} - \boldsymbol{U}^\star \boldsymbol{U}^{\star\top}$, thus $\boldsymbol{P}\boldsymbol{X}^\star = \boldsymbol{0}$. Recall that $\|\boldsymbol{P}\boldsymbol{U}\| = \delta^{(t)}$, $\tilde{\boldsymbol{U}}^+ = \boldsymbol{U} - \eta\text{GradU}$, and $\boldsymbol{U}^+ = \tilde{\boldsymbol{U}}^+ \boldsymbol{R}^{+-1}$ where $\tilde{\boldsymbol{U}}^+ \overset{\text{QR}}{=} \boldsymbol{U}^+\boldsymbol{R}^+$. We have

$$\begin{aligned}
\delta^{(t+1)} &= \text{SD}_2(\boldsymbol{U}^+, \boldsymbol{U}^\star) = \|\boldsymbol{P}\boldsymbol{U}^+\| \\
&\leq \|\boldsymbol{P}\tilde{\boldsymbol{U}}^+\| \cdot \|(\boldsymbol{R}^+)^{-1}\| = \|\boldsymbol{P}\tilde{\boldsymbol{U}}^+\| / \sigma_{\min}(\tilde{\boldsymbol{U}}^+) \\
&\leq \frac{\|\boldsymbol{P}(\boldsymbol{U} - \eta\mathbb{E}[\text{GradU}] + \eta\mathbb{E}[\text{GradU}] - \eta\text{GradU})\|}{(1 - \eta\|\text{GradU}\|)} \\
&\leq \frac{\|\boldsymbol{P}(\boldsymbol{U} - \eta p(\boldsymbol{U}\boldsymbol{B} - \boldsymbol{X}^\star)\boldsymbol{B}^\top)\| + \eta\|\mathbb{E}[\text{GradU}] - \text{GradU})\|}{(1 - \eta\|\mathbb{E}[\text{GradU}]\| - \eta\|\mathbb{E}[\text{GradU}] - \text{GradU}\|)} \\
&\leq \frac{\|\boldsymbol{P}\boldsymbol{U}\| \cdot \|(\boldsymbol{I} - \eta p\boldsymbol{B}\boldsymbol{B}^\top)\| + \eta\|\mathbb{E}[\text{GradU}] - \text{GradU})\|}{(1 - \eta\|\mathbb{E}[\text{GradU}]\| - \eta\|\mathbb{E}[\text{GradU}] - \text{GradU}\|)}.
\end{aligned} \tag{4}$$

Since $\delta^{(t)} \leq c/(\sqrt{r}\kappa^2)$, using the induction assumption and Lemma A.3, $\sigma_{\min}(\boldsymbol{B}) \geq 0.9\sigma^*_{\min}$ and $\|\boldsymbol{B}\| \leq 1.1\sigma^*_{\max}$. Using these, if $\eta \leq 0.5/(p\sigma^{*2}_{\max})$, then $\boldsymbol{I} - \eta p\boldsymbol{B}\boldsymbol{B}^\intercal$ is positive semi-definite (psd) and $\|\boldsymbol{I} - \eta p\boldsymbol{B}\boldsymbol{B}^\intercal\| \leq 1 - 0.8\eta p\sigma^{*2}_{\min}$ (see details in proof of Lemma A.6). Using this and the bounds from Lemma A.5 in (4), and using $1/(1-x) \leq 1 + 2x$ for $x < 0.5$,

$$\begin{aligned}
\delta^{(t+1)} &\leq \frac{\delta^{(t)}\left(1 - 0.8\eta p\sigma^{*2}_{\min} + 0.1\eta p\sigma^{*2}_{\min}\right)}{1 - \delta^{(t)}\left((1+\epsilon)\eta p\sqrt{r}\sigma^{*2}_{\max}\right)} \\
&\leq \delta^{(t)}(1 - 0.7\eta p\sigma^{*2}_{\min})(1 + 2\delta^{(t)}((1+\epsilon)\eta p\sqrt{r}\sigma^{*2}_{\max})) \\
&\leq \delta^{(t)}(1 - 0.7\eta p\sigma^{*2}_{\min} + \delta^{(t)} \cdot 2(1+\epsilon)\eta p\sqrt{r}\sigma^{*2}_{\max}) \\
&\leq \delta^{(t)}(1 - \eta p\sigma^{*2}_{\min}(0.7 - \delta^{(t)}2(1+\epsilon)\sqrt{r}\kappa^2)) \\
&\leq \delta^{(t)}(1 - \eta p\sigma^{*2}_{\min}(0.7 - 0.1))
\end{aligned}$$

The last row used $\delta^{(t)} \leq 0.1/(\sqrt{r}\kappa^2)$. Setting $\eta = 0.5/(p\sigma^{*2}_{\max})$, $\delta^{(t+1)} \leq (1 - 0.3/\kappa^2)\delta^{(t)}$. Using this and the induction assumption, $\delta^{(t+1)} \leq c/\sqrt{r}\kappa^2$. Thus claim (i) holds. Using Lemmas A.2 and A.4, claims (iii) and (iv) hold.

# Appendix B
# Proofs of Corollary 4.2 and the Lemmas

## A. *Proof of Corollary 4.2*

*Proof.* By Lemma A.1, if $p \geq C\kappa^6(\mu)^4 r^6/n$, then $\delta^{(0)} \leq c/(\sqrt{r}\kappa^2)$ and $\boldsymbol{U}^{(0)}$ is $\mu\sqrt{r}$-incoherent. Applying the Theorem for each $t = 1, 2, \ldots, T$, we can conclude that if $p \geq C\kappa^6(\mu)^4 r^{4.5}(r^{1.5} + T)/n$, then $\text{SD}_2(\boldsymbol{U}^{(T)}, \boldsymbol{U}^*) \leq (1 - 0.5/\kappa^2)^T \cdot c/(\sqrt{r}\kappa^2)$. Using the value of $T$, this right hand side is below $\epsilon$. The bound on $\|\boldsymbol{X}^{(T)} - \boldsymbol{X}^\star\|_F$ then follows using Lemmas A.2 and A.3. □

## B. *Brief proof ideas*

Lemma A.3 is proved below.

Lemma A.4 follows by writing $\boldsymbol{b}_k = (\boldsymbol{U}_k^\intercal \boldsymbol{U}_k)(\boldsymbol{U}_k^\intercal \boldsymbol{U}_k^*)\boldsymbol{b}_k^*$ applying the Matrix-Bernstein inequality twice to bound $\|\boldsymbol{U}_k^\intercal \boldsymbol{U}_k\|$ and $\boldsymbol{U}_k^\intercal \boldsymbol{U}_k^*$. See section B-F.

Lemma A.5: For 1), we use the Matrix Bernstein inequality, see section B-D. For 2), note that $\mathbb{E}[\text{GradU}] = p(\boldsymbol{X} - \boldsymbol{X}^\star)\boldsymbol{B}^\intercal$ because the expectation is taken with respect to an independent set of samples at each iteration, i.e., sample splitting.

Lemma A.6: 1) follows by using the Matrix-Bernstein inequality. For 2), we write $\tilde{\boldsymbol{u}}^{j(t+1)} = \boldsymbol{u}^{j(t)} - \eta\text{Grad}\boldsymbol{u}^j \pm \mathbb{E}[\text{Grad}\boldsymbol{u}^j]$ and subsequently bounding $\|\boldsymbol{u}^{j\intercal(t+1)}\| \leq \|\boldsymbol{R}^{-1}\|\|\tilde{\boldsymbol{u}}^{j(t)}\|$. The proofs are provided in Section B-E.

## C. *Proof of Lemma A.3*

Writing $\boldsymbol{X}^\star = \boldsymbol{U}\boldsymbol{G} + (\boldsymbol{I} - \boldsymbol{U}\boldsymbol{U}^\intercal)\boldsymbol{X}^\star$, and $\boldsymbol{X} = \boldsymbol{U}\boldsymbol{B}$, we have $\|\boldsymbol{X}^\star - \boldsymbol{X}\|_F \leq \|\boldsymbol{B} - \boldsymbol{G}\|_F + \|(\boldsymbol{I} - \boldsymbol{U}\boldsymbol{U}^\intercal)\boldsymbol{U}^*\boldsymbol{B}^*\|_F \leq \|\boldsymbol{B} - \boldsymbol{G}\|_F + \|(\boldsymbol{I} - \boldsymbol{U}\boldsymbol{U}^\intercal)\boldsymbol{U}^*\|_F\|\boldsymbol{B}^*\| \leq \delta^{(t)}\sqrt{r}\sigma^*_{\max} + \delta^{(t)}\sqrt{r}\sigma^*_{\max}$.

For the second part, using the bound on $\|\boldsymbol{B} - \boldsymbol{G}\|$, $\|\boldsymbol{B}\| = \|\boldsymbol{B} - \boldsymbol{G} + \boldsymbol{G}\| \leq \|\boldsymbol{B} - \boldsymbol{G}\| + \|\boldsymbol{G}\| \leq \delta^{(t)}\sqrt{r}\sigma^*_{\max} + \sigma^*_{\max}$.

For the third part, $\sigma_{\min}(\boldsymbol{B}) \geq \sigma_{\min}(\boldsymbol{G}) - \sigma_{\max}(\boldsymbol{B} - \boldsymbol{G}) \geq \sqrt{1 - \delta^{(t)2}}\sigma_{\min} - \delta^{(t)}\sqrt{r}\sigma^*_{\max}$, where $\sigma_{\min}(\boldsymbol{G}) = \sigma_{\min}(\boldsymbol{U}^\intercal \boldsymbol{U}^* \boldsymbol{B}^*) \geq \sigma_{\min}(\boldsymbol{U}^\intercal \boldsymbol{U}^*)\sigma^*_{\min} \geq \sqrt{1 - \delta^{(t)2}}\sigma^*_{\min}$.

### D. Proof of Lemma A.5

The gradient with respect to $\boldsymbol{U}$ is $\mathrm{GradU} = \sum_{jk} \xi_{jk} \boldsymbol{e}_j (\boldsymbol{x}_{jk} - \boldsymbol{x}^*_{jk}) \boldsymbol{b}_k^\intercal$. We will bound $\|\mathrm{GradU}\|$ by the Matrix-Bernstein inequality. Using $n \le q$ and (5),

$$L = \max_{jk} |\boldsymbol{x}_{jk} - \boldsymbol{x}^\star_{jk}| \max_k \|\boldsymbol{b}_k\| \le 2\mu_u (r/\sqrt{n}) \delta^{(t)} \sigma^*_{\max} \cdot \mu \sqrt{r/q} \sigma^*_{\max} \le 2\mu_u \mu (r^{3/2}/n) \delta^{(t)} {\sigma^*_{\max}}^2,$$

where $\max_{jk} |\boldsymbol{x}_{jk} - \boldsymbol{x}^*_{jk}|$ is bounded below

$$|\boldsymbol{e}_j^\top (\boldsymbol{X} - \boldsymbol{X}^\star) \boldsymbol{e}_k| \le \|\boldsymbol{e}_j^\top \boldsymbol{U}\| \|\boldsymbol{B} - \boldsymbol{G}\| + \|(\boldsymbol{U}\boldsymbol{U}^\top - \boldsymbol{I}) \boldsymbol{U}^\star\| \|\boldsymbol{B}^\star \boldsymbol{e}_k\| \le \mu_u \sqrt{r/n} \sqrt{r} \delta^{(t)} \sigma^*_{\max} + \mu \sqrt{r/q} \delta^{(t)} \sigma^*_{\max} \le 2\mu_u (r/\sqrt{n}) \delta^{(t)} \sigma^*_{\max}. \quad (5)$$

The variances are

$$\sigma_1^2 = p \sum_{jk} (\boldsymbol{x}_{jk} - \boldsymbol{x}^\star_{jk})^2 \boldsymbol{e}_j \boldsymbol{b}_k^\top \boldsymbol{b}_k \boldsymbol{e}_j^\top \le p \|\boldsymbol{b}_k\|^2 \|\boldsymbol{X} - \boldsymbol{X}^\star\|_F^2 \le p\mu^2 (r/q) {\sigma^*_{\max}}^2 \cdot (\delta^{(t)} \sqrt{r} \sigma^*_{\max})^2 = p\mu^2 (r^2/q) \delta^{(t)2} {\sigma^*_{\max}}^4.$$

$$\sigma_2^2 = p \| \sum_{jk} (\boldsymbol{x}_{jk} - \boldsymbol{x}^\star_{jk})^2 \boldsymbol{e}_j^\top \boldsymbol{e}_j \boldsymbol{b}_k \boldsymbol{b}_k^\top \| \le p \|\boldsymbol{b}_k\|^2 \|\boldsymbol{X} - \boldsymbol{X}^\star\|_F^2 = \sigma_1^2.$$

Setting $t = \epsilon p \sqrt{r} \delta^{(t)} {\sigma^*_{\max}}^2$, we have

$$\frac{t^2}{\sigma^2} = \frac{\epsilon^2 p^2 r \delta^{(t)2} {\sigma^*_{\max}}^4}{p\mu^2 (r^2/q) \delta^{(t)2} {\sigma^*_{\max}}^4} = \frac{\epsilon^2 pq}{\mu^2 r} \le \frac{\epsilon^2 pq}{\mu_u \mu r}, \quad \frac{t}{L} = \frac{\epsilon p \sqrt{r} \delta^{(t)} {\sigma^*_{\max}}^2}{\mu_u \mu (r^{3/2}/n) \delta^{(t)} {\sigma^*_{\max}}^2} = \frac{\epsilon p n}{\mu_u \mu r}.$$

By matrix Bernstein, for $\epsilon \le 1$, w.p. at least $1 - \exp(\log q - \epsilon^2 pn/\mu_u \mu r)$,

$$\|\mathrm{GradU} - \mathbb{E}[\mathrm{GradU}]\| \le \epsilon p \sqrt{r} \delta^{(t)} {\sigma^*_{\max}}^2.$$

If $p > \mu_u \mu r \max(\log q, \log n)/n\epsilon^2$, then the above bound holds w.p. at least $1 - 1/n^3$. Also,

$$\mathbb{E}[\mathrm{GradU}] = p(\boldsymbol{X} - \boldsymbol{X}^\star) \boldsymbol{B}^\top,$$

### E. Proof of Lemma A.6

Let $\mathrm{Grad}\boldsymbol{u}^j \in \mathbb{R}^{1\times r}$ denote the gradient of $\boldsymbol{U} \in \mathbb{R}^{n \times r}$ with respect to row $j$. We note the following

$$\mathrm{Grad}\boldsymbol{u}^j = \sum_k \xi_{jk} (\boldsymbol{x}_{jk} - \boldsymbol{x}^\star_{jk}) \boldsymbol{b}_k^\top, \ \|\mathbb{E}[\mathrm{GradU}_j]\| \lesssim 2p \|\boldsymbol{u}^j\| {\sigma^*_{\max}}^2.$$

$$L = \max_k |\boldsymbol{x}_{jk} - \boldsymbol{x}^\star_{jk}| \max_k \|\boldsymbol{b}_k\| \le \max(\max_k |\boldsymbol{x}_{jk}|, \max_k |\boldsymbol{x}^\star_{jk}|) \max_k \|\boldsymbol{b}_k\| \le \max(\|\boldsymbol{u}^j\|, \|\boldsymbol{u}^{*j}\|) \mu^2 (r/q) {\sigma^*_{\max}}^2.$$

$$\sigma_1^2 = \| \sum_k p(\boldsymbol{x}_{jk} - \boldsymbol{x}^\star_{jk})^2 \boldsymbol{b}_k^\top \boldsymbol{b}_k \| \le 2p \| \sum_k {\boldsymbol{u}^j}^\top \boldsymbol{b}_k \boldsymbol{b}_k^\top \boldsymbol{u}^j \boldsymbol{b}_k^\top \boldsymbol{b}_k \| \le 2p \max_k \|\boldsymbol{b}_k\|^2 {\boldsymbol{u}^j}^\top (\sum_k \boldsymbol{b}_k \boldsymbol{b}_k^\top) \boldsymbol{u}^j \le 2p \|\boldsymbol{u}^j\|^2 \mu^2 (r/q) {\sigma^*_{\max}}^4.$$

$$\sigma_2^2 = \| \sum_k p(\boldsymbol{x}_{jk} - \boldsymbol{x}^\star_{jk})^2 \boldsymbol{b}_k \boldsymbol{b}_k^\top \| \le 2p \| \sum_k {\boldsymbol{u}^j}^\top \boldsymbol{b}_k \boldsymbol{b}_k^\top \boldsymbol{u}^j \boldsymbol{b}_k \boldsymbol{b}_k^\top \| \le 2p \max_k \|\boldsymbol{b}_k\|^2 \|{\boldsymbol{u}^j}^\top (\sum_k \boldsymbol{b}_k \boldsymbol{b}_k^\top) \boldsymbol{u}^j \| \le 2p \|\boldsymbol{u}^j\|^2 \mu^2 (r/q) {\sigma^*_{\max}}^4.$$

Here, $\sigma_1^2 \equiv \mathbb{E}[\sum_k \xi_{jk} (\boldsymbol{x}_{jk} - \boldsymbol{x}^*_{jk})^2 \boldsymbol{b}_k^\intercal \boldsymbol{b}_k]$ and $\sigma_2^2 \equiv \mathbb{E}[\sum_k \xi_{jk} (\boldsymbol{x}_{jk} - \boldsymbol{x}^*_{jk})^2 \boldsymbol{b}_k \boldsymbol{b}_k^\intercal]$. By the matrix Bernstein inequality with $t = \epsilon p \|\boldsymbol{u}^j\| {\sigma^*_{\min}}^2$, we have w.p. at least $1 - \exp(\log q - \epsilon^2 pn/\mu^2 \kappa^4 r)$,

$$\|\mathbb{E}[\mathrm{GradU}_j] - \mathrm{GradU}_j\| \le \epsilon p \|\boldsymbol{u}^j\| {\sigma^*_{\min}}^2.$$

This completes the proof for the first part of the lemma.

By line 5 of Algorithm 1, adding/subtracting $\mathbb{E}[\mathrm{GradU}_j] = p {\boldsymbol{u}^{*j}}^\top \boldsymbol{B}^\star \boldsymbol{B}^\top$, and using the above bound on $\|\mathbb{E}[\mathrm{GradU}_j] - \mathrm{GradU}_j\|$

$$\tilde{\boldsymbol{u}}_j^{(t+1)^\top} = \boldsymbol{u}^{j(t)\top} (\boldsymbol{I} - \eta p \boldsymbol{B}\boldsymbol{B}^\top) - \eta \mathrm{GradU}_j = \boldsymbol{u}^{j(t)\top} (\boldsymbol{I} - \eta p \boldsymbol{B}\boldsymbol{B}^\top) - \eta p {\boldsymbol{u}^{*j}}^\top \boldsymbol{B}^\star \boldsymbol{B}^\top + \eta (\mathbb{E}[\mathrm{GradU}_j] - \mathrm{GradU}_j),$$

w.p. at least $1 - \exp(\log q - \epsilon^2 pn/\mu^2 \kappa^4 r)$.

Using the assumed bound on $\boldsymbol{B} - \boldsymbol{G}$ and Lemma A.3 and $\delta^{(t)} \le c/\sqrt{r}\kappa^2$, $\sigma_{\min}(\boldsymbol{B}) \ge 0.9\sigma^*_{\min}$ and $\sigma_{\max}(\boldsymbol{B}) \le 1.1\sigma^*_{\max}$. Thus, if $\eta < 0.5/p{\sigma^*_{\max}}^2$ then, $\boldsymbol{I} - \eta p \boldsymbol{B}\boldsymbol{B}^\top$ is positive semi-definite (psd) and $\|\boldsymbol{I} - \eta p \boldsymbol{B}\boldsymbol{B}^\top\| = 1 - \eta p \sigma^2_{\min}(\boldsymbol{B}) \le 1 - 0.9\eta p {\sigma^*_{\min}}^2$. Thus, if $\eta < 0.5/p{\sigma^*_{\max}}^2$, then,

$$\|\tilde{\boldsymbol{u}}_j^{(t+1)}\| \le \|\boldsymbol{u}^{j(t)}\| (1 - 0.9\eta p {\sigma^*_{\min}}^2) + \epsilon \eta p {\sigma^*_{\min}}^2 \|\boldsymbol{u}^{j(t)}\| + 1.1\eta p \|\boldsymbol{u}^{*j}\| {\sigma^*_{\max}}^2 \le (1 - (0.9 - \epsilon)\eta p {\sigma^*_{\min}}^2) \|\boldsymbol{u}^{j(t)}\| + \eta p {\sigma^*_{\max}}^2 \|\boldsymbol{u}^{*j}\|. \quad (6)$$

w.p. at least $1 - \exp(\log q - \epsilon^2 pn/\mu^2 \kappa^4 r)$.

We bound $\|{\boldsymbol{u}^j}^{\intercal(t+1)}\| \le \|(\boldsymbol{R}^{(t+1)})^{-1}\| \cdot \|\tilde{\boldsymbol{u}}_j^{\intercal(t+1)}\|$, where $\tilde{\boldsymbol{U}}^{(t+1)} \overset{\mathrm{QR}}{=} \boldsymbol{U}^{(t+1)} \boldsymbol{R}^{(t+1)}$, and

$$\|(\boldsymbol{R}^{(t+1)})^{-1}\| = 1/(\sigma_{\min}(\boldsymbol{U} - \eta \|\mathrm{GradU}\|) \le 1/(1 - \eta p (1+\epsilon) \sqrt{r} \delta^{(t)} \sigma^{*2}_{\max}) \le 1/(1 - 0.25\eta p {\sigma^*_{\min}}^2) \le 1 + 0.5\eta p {\sigma^*_{\min}}^2. \quad (7)$$

w.p. given in Lemma A.5. In the above we have used Lemma A.5 and the upper bound on $\delta^{(t)}$. Thus,

$$\begin{aligned}\|\boldsymbol{u}_j^{(t+1)}\| &\leq (1+0.5\eta p{\sigma^*_{\min}}^2)(1-(0.9-\epsilon)\eta p{\sigma^*_{\min}}^2)\|{\boldsymbol{u}^j}^{(t)}\| + (1+0.5\eta p{\sigma^*_{\min}}^2)\eta p{\sigma^*_{\max}}^2\|\boldsymbol{u}^{*j}\| \\ &\leq (1-(0.4-\epsilon)\eta p{\sigma^*_{\min}}^2)\|{\boldsymbol{u}^j}^{(t)}\| + (1+0.5\eta p{\sigma^*_{\min}}^2)\eta p{\sigma^*_{\max}}^2\|\boldsymbol{u}^{*j}\| \\ &\leq (1-(0.4-\epsilon)\eta p{\sigma^*_{\min}}^2)\|{\boldsymbol{u}^j}^{(t)}\| + (1+0.25/\kappa^2)0.5\|\boldsymbol{u}^{*j}\| \\ &\leq (1-\frac{0.15}{\kappa^2})\|{\boldsymbol{u}^j}^{(t)}\| + 0.7\|\boldsymbol{u}^{*j}\|\end{aligned}$$

where the last bound follows by setting $\eta = 0.5/p{\sigma^*_{\max}}^2$, $\epsilon = 0.1$.

Thus, we have shown that if $\delta^{(t)} \leq c/\sqrt{r}\kappa^2$, and $\eta = 0.5/p{\sigma^*_{\max}}^2$, w.p. at least $1-3/n^3$,

$$\|{\boldsymbol{u}^j}^{(t+1)}\| \leq (1-\frac{0.15}{\kappa^2})\|{\boldsymbol{u}^j}^{(t)}\| + 0.7\|\boldsymbol{u}^{*j}\|$$

if $p$ satisfies the stated bound in the lemma.

### F. Proof of Lemma A.4

We have

$$\boldsymbol{b}_k = \underbrace{(\boldsymbol{U}_k^\intercal \boldsymbol{U}_k)^{-1}}_{T_1} \underbrace{\boldsymbol{U}_k^\intercal \boldsymbol{U}_k^*}_{T_2} \boldsymbol{b}_k^*. \tag{8}$$

The following has been proved in Lemma C.6 of [2]. If $p \geq C\frac{\mu_u^2 r}{n\epsilon^2}(\log n + \log r)$, then with probability greater than $1-\frac{1}{n^3}$,

$$\|(\boldsymbol{U}_k^\intercal \boldsymbol{U}_k)^{-1}\| \leq \frac{1}{(1-\epsilon)p}. \tag{9}$$

Consider the second term, $T_2$. The term $\|T_2 - \mathbb{E}[T_2]\|$ can be bounded by the Matrix-Bernstein inequality. We have $\mathbb{E}[T_2] = p\boldsymbol{U}^\intercal\boldsymbol{U}^* \neq p\boldsymbol{I}$. By the reverse triangle inequality,

$$\|\boldsymbol{U}_k^\intercal \boldsymbol{U}_k^* - p\boldsymbol{U}^\intercal\boldsymbol{U}^*\| \geq \|\boldsymbol{U}_k^\intercal \boldsymbol{U}_k^*\| - p, \tag{10}$$

where we have used $\|\boldsymbol{U}^\intercal\boldsymbol{U}^*\| \leq \|\boldsymbol{U}\|\|\boldsymbol{U}^*\| \leq 1$. Therefore,

$$\|\boldsymbol{U}_k^\intercal \boldsymbol{U}_k^*\| \leq \|\boldsymbol{U}_k^\intercal \boldsymbol{U}_k^* - p\boldsymbol{U}^\intercal\boldsymbol{U}^*\|_{op} + p. \tag{11}$$

The second difference from the proof of (9) is that $T_2 - \mathbb{E}[T_2]$ is not symmetric. The variance $\sigma^2$ is now

$$\sigma^2 = \max(\|\sum_j \mathbb{E}[\boldsymbol{Z}_j\boldsymbol{Z}_j^\intercal]\|, \|\sum_j \mathbb{E}[\boldsymbol{Z}_j^\intercal\boldsymbol{Z}_j]\|),$$

where $\boldsymbol{Z}_j = (\xi_{jk}-p)\boldsymbol{u}^j{\boldsymbol{u}^j}^{*\intercal}$, and

$$\begin{aligned}&\mathbb{E}[\boldsymbol{Z}_j] = 0, \\ &\|\boldsymbol{Z}_j\| = \max(1-p,p)\|\boldsymbol{u}^j\|\|{\boldsymbol{u}^j}^*\| \leq \mu_u\mu\frac{r}{n}, \\ &\boldsymbol{Z}_j\boldsymbol{Z}_j^\intercal \sim \begin{cases}(1-p)^2\|{\boldsymbol{u}^j}^*\|^2\boldsymbol{u}^j{\boldsymbol{u}^j}^\intercal & \text{w.p. } p \\ p^2\|{\boldsymbol{u}^j}^*\|^2\boldsymbol{u}^j{\boldsymbol{u}^j}^\intercal & \text{w.p. } 1-p,\end{cases} \\ &\boldsymbol{Z}_j^\intercal\boldsymbol{Z}_j \sim \begin{cases}(1-p)^2\|\boldsymbol{u}^j\|^2{\boldsymbol{u}^j}^*{\boldsymbol{u}^j}^{*\intercal} & \text{w.p. } p \\ p^2\|\boldsymbol{u}^j\|^2{\boldsymbol{u}^j}^*{\boldsymbol{u}^j}^{*\intercal} & \text{w.p. } 1-p,\end{cases}\end{aligned}$$

Both variances $\sigma^2(\boldsymbol{Z}_j\boldsymbol{Z}_j^\intercal)$ and $\sigma^2(\boldsymbol{Z}_j^\intercal\boldsymbol{Z}_j)$ can be bounded by the same upper bound. Note that

$$\begin{aligned}\mathbb{E}[\boldsymbol{Z}_j\boldsymbol{Z}_j^\intercal] &= p(1-p)^2\|\boldsymbol{u}^{*j}\|^2\boldsymbol{u}^j{\boldsymbol{u}^j}^\intercal + p^2(1-p)\|\boldsymbol{u}^{*j}\|^2\boldsymbol{u}^j{\boldsymbol{u}^j}^\intercal \\ &\triangleq p'\|{\boldsymbol{u}^j}^*\|^2\boldsymbol{u}^j{\boldsymbol{u}^j}^\intercal, \quad \text{where } p' = p(1-p)^2 + p^2(1-p) \leq 2p.\end{aligned} \tag{12}$$

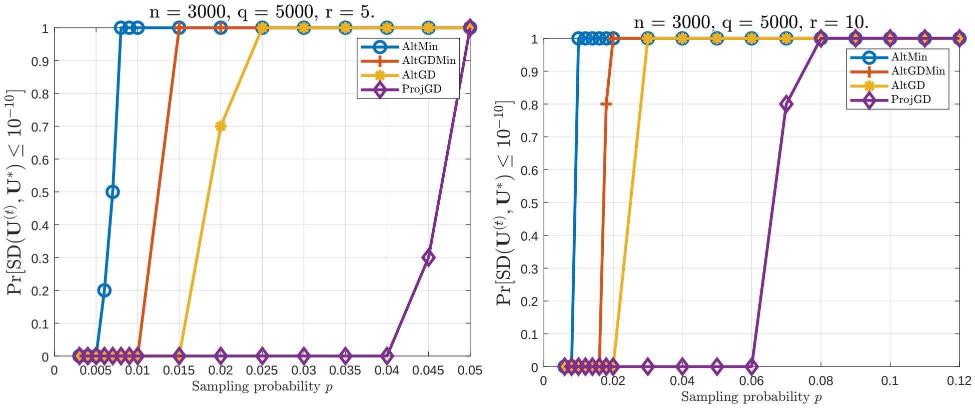


(a)

Fig. 2: Sample complexity comparison of AltGDMin with that of benchmark methods using phase transition plots. We plot a Monte Carlo estimate of the probability of the recovery error being below $10^{-10}$ for different values of $p$ (the probability of any entry of $\boldsymbol{X}^\star$ being observed).

The variance $\sigma^2(\boldsymbol{Z}_j\boldsymbol{Z}_j^\intercal)$ is

$$\begin{aligned}
\sigma^2(\boldsymbol{Z}_j\boldsymbol{Z}_j^\intercal) &= \|\sum_{j=1}^{j=n}\mathbb{E}[\boldsymbol{Z}_j\boldsymbol{Z}_j^\intercal]\| = p'\|\sum_{j=1}^{j=n}\|\boldsymbol{u}^{j*}\|^2(\boldsymbol{u}^j\boldsymbol{u}^{j\intercal})\| \\
&= p'\max_{\boldsymbol{w}:\,\|\boldsymbol{w}\|=1}\sum_{j=1}^{j=n}\boldsymbol{w}^\intercal(\|\boldsymbol{u}^{j*}\|^2\boldsymbol{u}^j\boldsymbol{u}^{j\intercal})\boldsymbol{w} \\
&\leq p'\mu^2\frac{r}{n}\max_{\boldsymbol{w}:\,\|\boldsymbol{w}\|=1}\boldsymbol{w}^\intercal\sum_{j=1}^{j=n}\boldsymbol{u}^j\boldsymbol{u}^{j\intercal}\boldsymbol{w} \\
&\leq p'\mu^2\frac{r}{n}\max_{\boldsymbol{w}:\,\|\boldsymbol{w}\|=1}\boldsymbol{w}^\intercal\boldsymbol{U}^\intercal\boldsymbol{U}\boldsymbol{w} \\
&= p'\mu^2\frac{r}{n}\max_{\boldsymbol{w}}\boldsymbol{w}^\intercal\boldsymbol{w} \\
&= p'\mu^2\frac{r}{n} \leq 2p\mu^2\frac{r}{n}.
\end{aligned}$$

$\sigma^2(\boldsymbol{Z}_j^\intercal\boldsymbol{Z}_j)$ can be similarly bounded as $\sigma^2(\boldsymbol{Z}_j^\intercal\boldsymbol{Z}_j) \leq 2p\mu_u^2\frac{r}{n}$. Because $\mu_u \geq \mu$, we have $\sigma^2(\boldsymbol{Z}_j\boldsymbol{Z}_j^\intercal) \geq \sigma^2(\boldsymbol{Z}_j^\intercal\boldsymbol{Z}_j)$. By the Matrix-Bernstein inequality, for $\epsilon \leq 2$ and w.p. greater than $1-\exp(\log 2r - c\frac{n\epsilon^2 p}{\mu_u^2 r})$

$$\|\boldsymbol{U}_k^\intercal\boldsymbol{U}_k^* - p\boldsymbol{U}^\intercal\boldsymbol{U}^*\| \leq \epsilon p. \tag{13}$$

From (11) and (13), w.h.p,

$$\|\boldsymbol{U}_k^\intercal\boldsymbol{U}_k^*\| \leq (1+\epsilon)p. \tag{14}$$

Substituting (9), (14) in (8), and setting $\epsilon = 1/10$, we have

$$\|\boldsymbol{b}_k\| \leq \frac{3}{2}\|\boldsymbol{b}_k^*\| \leq \frac{3}{2}\sigma_{\max}^*\mu\sqrt{r/q}. \tag{15}$$

## Appendix C
## More Simulation Experiments

AltGDMin is compared with benchmark methods based on sample complexity, that is, the number of observed entries required for successful matrix completion. We plot a Monte Carlo estimate of the probability of the recovery error being below $10^{-10}$ for different values of $p$ (the probability of any entry of $\boldsymbol{X}^\star$ being observed).
